# Supplementary material for: Dynamics-Guided Diffusion Model for Sensor-less Robot Manipulator Design
Source: arXiv:2402.15038 source file (2025-03-28)
Supplement: Supplementary file 1 [file appendix.tex]

\section*{Appendix}
\setcounter{section}{0}

\section{Tasks and metrics}
We provide more details about the evaluation manipulation tasks, and introduce more metrics for each task in this section.

    Primitive objectives:
    \begin{itemize}

        \item \textbf{Shift up}: Make the object shift upward (along the negative x-axis) under all initial poses. Metrics are the average success rate after one closure $S_x^-\uparrow(\%)$, average delta translation along the x-axis after one closure $\Delta x\downarrow(cm)$, and average final x coordinate after the 40th gripper closure $x\downarrow(cm)$. The metrics are averaged among trajectories with different initial \textcolor{red}{object} poses. The motion objective is $f(o,m,p)=-\Delta x(o,m,p)$, then the design objective can be aggregated from $f(o,m,p)$ as $F(m)=\sum_{o}\sum_{p} f(o,m,p)$.
        \item \textbf{Shift down}: Make the object shift downward (along the positive x-axis) under all initial poses. Metrics are average success rate $S_x^+\uparrow(\%)$, average delta translation along the x-axis $\Delta x\uparrow(cm)$, and average final x coordinate $x\uparrow(cm)$. The motion objective is $f(o,m,p)=\Delta x(o,m,p)$.
        \item \textbf{Shift left}: Make the object shift leftward (along the negative y-axis) under all initial poses. Metrics are average success rate $S_y^-\uparrow(\%)$, average delta translation along the y-axis $\Delta y\downarrow(cm)$, and average final y coordinate $y\downarrow(cm)$. The motion objective is $f(o,m,p)=-\Delta y(o,m,p)$.
        \item \textbf{Shift right}: Make the object shift rightward (along the positive y-axis) under all initial poses. Metrics are average success rate $S_y^+\uparrow(\%)$, average delta translation along the y-axis $\Delta y\uparrow(cm)$, and average final y coordinate $y\uparrow(cm)$. The motion objective is $f(o,m,p)=\Delta y(o,m,p)$.
        \item \textbf{Rotate clockwise}: Make the object rotate clockwise (negative delta rotation around the z-axis) under all initial poses. Metrics are average success rate $S_\theta^-\uparrow(\%)$, average delta rotation around the z-axis $\Delta \theta\downarrow(\degree)$, and average final orientation $\theta\downarrow(\degree)$. The motion objective is $f(o,m,p)=-\Delta \theta(o,m,p)$.
        \item \textbf{Rotate counterclockwise}: Make the object rotate counterclockwise (positive delta rotation around the z-axis) under all initial poses. Metrics are average success rate $S_\theta^+\uparrow(\%)$, average delta rotation around the z-axis $\Delta \theta\uparrow(\degree)$, and average final orientation $\theta\uparrow(\degree)$. The motion objective is $f(o,m,p)=\Delta \theta(o,m,p)$.
    \end{itemize}

    Complex objectives:
    \begin{itemize}
        \item \textbf{Rotate}: Make the object rotate either clockwise or counterclockwise under all initial poses. The metrics are average success rate $S_\theta^{+-}\uparrow(\%)$, the average absolute value of delta rotation around the z-axis $|\Delta \theta|\downarrow(\degree)$, and the average absolute value of final orientation $|\theta|\downarrow(\degree)$. The motion objective is $f(o,m,p)=[\Delta \theta(o,m,p)]^2$.

        \item \textbf{Rotate clockwise and shift up}: Make the object rotate clockwise and shift up under all initial poses. The metrics are average success rate $S_\theta^-\&S_x^-\uparrow(\%)$, average delta rotation around the z-axis $\Delta \theta\downarrow(\degree)$, average final orientation $\theta\downarrow(\degree)$, average delta translation along the x-axis after one closure $\Delta x\downarrow(cm)$, and average final x coordinate after the 40th closure $x\downarrow(cm)$.
        The motion objective is $f(o,m,p)=-\Delta \theta(o,m,p)-\Delta x(o,m,p)$.

        \item \textbf{Rotate clockwise and shift left}: Make the object rotate clockwise and shift left under all initial poses.
        The metrics are average success rate $S_\theta^-\&S_y^-\uparrow(\%)$, average delta rotation around the z-axis $\Delta \theta\downarrow(\degree)$, average final orientation $\theta\downarrow(\degree)$, average delta translation along the y-axis $\Delta y\downarrow(cm)$, and average final y coordinate $y\downarrow(cm)$.
        The motion objective is $f(o,m,p)=-\Delta \theta(o,m,p)-\Delta y(o,m,p)$.

        \item \textbf{Convergence}: Make the object always end in a fixed final pose under a range of initial poses.
        % Convergence is useful because it is often necessary to reorient parts before assembly in manufacturing~\cite{goldberg1993orienting}, and reorienting objects to a fixed pose can induce a more stable grasp, especially when no sensor is available or the pose estimation is very inaccurate. Previous work~\cite{aceituno2023certified,goldberg1993orienting,zhang2002gripper} tackles convergence with manual or analytical designs of policy or hardware, and only deals with planar polygonal objects. Our framework enables automatically generating manipulators that achieve good convergence for any 2D or 3D shape. 
        % The objective is to make the object rotate towards the convergence pose, encouraging the object to rotate in the positive direction when its initial orientation is smaller than the target orientation, or else rotate in the negative direction. We first forward the dynamics network with the unguided generated shape to get a pseudo profile, determine the largest convergence range and its corresponding convergence target pose, and guide the diffusion generation with the gradient of the design objective. 
        The metric is the maximum convergence range $R_c^{max}\uparrow(\degree)$, the largest range of initial orientations leading to a consistent final orientation within a small tolerance. We report the maximum convergence range within the tolerance of $3\degree$, $5\degree$, and $10\degree$, respectively.

              % \item \textbf{Multi-object sorting}:
    \end{itemize}

% \huy{TODO: success thresholds for different tasks}

\section{additional results}
We report results on all the tasks and metrics described above in Tab.~\ref{tab:prim_result}, Tab.~\ref{tab:comp_result}, Tab.~\ref{tab:multi_prim_result}, and Tab.~\ref{tab:multi_comp_result}. The evaluation procedure is the same as described in the main paper, where we run each approach 16 times per object-task pair and select the best performance, then average among test objects. \ours outperforms baselines consistently on both discrete metrics (\eg average success rate) and continuous metrics (\eg delta transformation and final transformation).

\begin{table*}
    \centering
    % \footnotesize
    \setlength\tabcolsep{3pt}
    \begin{tabular}{cc|ccc|ccc|ccc|ccc|ccc|ccc}
        \toprule
        % \multicolumn{2}{c}{} & \multicolumn{18}{c}{Primitive} & \multicolumn{12}{c}{Complex}\\
        \multicolumn{2}{c|}{} & \multicolumn{3}{c|}{up} & \multicolumn{3}{c|}{down} & \multicolumn{3}{c|}{left} & \multicolumn{3}{c|}{right} & \multicolumn{3}{c|}{clock} & \multicolumn{3}{c}{counter}                                                                                                                                                                                                                                                                  \\
        \multicolumn{2}{c|}{} & $S_x^-\uparrow$         & $\Delta x\downarrow$      & $x\downarrow$             & $S_x^+\uparrow$            & $\Delta x\uparrow$         & $x\uparrow$                 & $S_y^-\uparrow$ & $\Delta y\downarrow$ & $y\downarrow$ & $S_y^+\uparrow$ & $\Delta y\uparrow$ & $y\uparrow$ & $S_\theta^-\uparrow$ & $\Delta \theta\downarrow$ & $\theta\downarrow$ & $S_\theta^+\uparrow$ & $\Delta \theta\uparrow$ & $\theta\uparrow$        \\
        \midrule

        \multirow{3}{*}{2D}
                              & Unguided                    & 56.8                       & -0.2                      & -1.3                       & 82.1                        & 0.3                         & 1.9             & 82.9                  & -0.5          & -1.2            & 80.4                & 0.5         & 1.4                  & 46.9                       & -1.5               & -9.5                 & 58.5                     & 2.3              & 11.1  \\
                              & Opt.                     & 79.5                       & -0.4                      & -2.2                       & 53.3                        & 0.4                         & 2.3             & 81.3                  & -0.6          & -2.4            & 94.0                & 0.7         & 1.7                  & 48.8                       & \textbf{-2.9}               & -8.8                 & 73.2                     & 3.6              & 9.6 \\
                              & \ours                    & \textbf{88.2}                       & \textbf{-0.4}                      & \textbf{-3.1}                       & \textbf{92.0}                        & \textbf{0.5}                         & \textbf{3.7}             & \textbf{96.7}                  & \textbf{-0.7}          & \textbf{-2.4}            & \textbf{97.7}                & \textbf{0.8}         & \textbf{2.1}                  & \textbf{60.8}                       & -2.6               & \textbf{-12.3}                & \textbf{72.0}                     & \textbf{3.6}              & \textbf{14.2} \\
        \midrule

        \multirow{3}{*}{3D}
                              & Unguided                    & 43.0                       & -0.1                      & -0.6                       & 43.8                        & 0.1                         & 1.0             & 80.4                  & -0.2          & -1.2            & 87.9                & 0.2         & 0.9                  & 41.2                       & -1.1               & -4.9                 & 33.5                     & 0.5              & 2.7  \\
                              & Opt.                     & 47.4                       & -0.1                      & -1.3                       & 66.3                        & 0.2                         & 1.7            & 86.3                  & -0.3          & -1.3            & 88.1                & 0.3         & 1.6                  & 59.1                       & -1.9               & -5.0                 & 52.0                     & 1.2              & 4.6  \\
                              & \ours                    & \textbf{81.5}                       & \textbf{-0.2}                      & \textbf{-1.6}                       & \textbf{75.1}                        & \textbf{0.2}                         & \textbf{1.7}             & \textbf{95.1}                  & \textbf{-0.4}          & \textbf{-1.8}            & \textbf{97.2}                & \textbf{0.4}         & \textbf{1.9}                  & \textbf{69.9}                       & \textbf{-2.3}               & \textbf{-7.7}                & \textbf{65.0}                     & \textbf{2.2}              & \textbf{6.3} \\

        \bottomrule
    \end{tabular}
    \caption{Single Object Primitive Objectives Evaluation}
    \label{tab:prim_result}
\end{table*}

\begin{table*}
    \centering
    \footnotesize
    \setlength\tabcolsep{2pt}
    \begin{tabular}{cc|ccc|ccccc|ccccc|ccc}
        \toprule
        % \multicolumn{2}{c}{} & \multicolumn{18}{c}{Primitive} & \multicolumn{12}{c}{Complex}\\
        \multicolumn{2}{c|}{} & \multicolumn{3}{c|}{rotate} & \multicolumn{5}{c|}{clock-up} & \multicolumn{5}{c|}{clock-left} & \multicolumn{3}{c}{convergence}                                                                                                                                                                                                                                                                       \\
        \multicolumn{2}{c|}{} & $S_\theta^{+-}\uparrow$      & $|\Delta \theta|\uparrow$     & $|\theta|\uparrow$              & $S_\theta^-\&S_x^-\uparrow$            & $\Delta \theta\downarrow$ & $\theta\downarrow$ & $\Delta x\downarrow$ & $x\downarrow$ & $S_\theta^-\&S_y^+\uparrow$ & $\Delta \theta\downarrow$ & $\theta\downarrow$ & $\Delta y\downarrow$ & $y\downarrow$ & $R_c^{max}(3\degree)\uparrow$  & $R_c^{max}(5\degree)\uparrow$  & $R_c^{max}(10\degree)\uparrow$  \\
        \midrule
        \multirow{3}{*}{2D}
                              & Unguided                        & 74.0                            & 3.5                             & 18.2                            & 36.4                       & -1.5               & -9.5            & -0.2                  & -1.3          & 36.9                 & -1.5                       & -9.5               & -0.5            & -1.2                  & 56.5             & 61.7                   & 68.7 \\
                              & Opt.                         & 78.9                            & 4.5                             & 18.9                            & 29.3                       & -1.8               & -4.2            & -0.3                  & -1.0          & 49.4                 & -2.9                       & -9.0               & -0.6             & -2.1                  & 69.6          & 73.7                & 82.1  \\
                              & \ours                        & \textbf{79.3}                            & \textbf{4.5}                             & \textbf{20.1}                            & \textbf{62.7}                       & \textbf{-3.3}               & \textbf{-14.5}           & \textbf{-0.4}                  & \textbf{-3.6}          & \textbf{63.7}                 & \textbf{-3.2}                       & \textbf{-10.1}               & \textbf{-0.7}           & \textbf{-2.4}                  & \textbf{78.4}             & \textbf{83}                   & \textbf{89.3} \\
        \midrule

        \multirow{3}{*}{3D}
                              & Unguided                        & 64.2                             & 2.2                               & 16.5                               & 30.3                       & -1.1               & -4.9            & -0.1                  & -0.6          & 33.1                 &-0.5                         & -2.7                  & -0.2               & -1.2                   & 52.2             & 63.6                   & 67.8  \\
                              & Opt.                         & 66.9                            & 2.4                             & 15.7                            & 29.2                       & -1.1                & -2.7            & -0.1                  & -0.5          & 37.7                 & -1.3                       & -3.3               & -0.3            & -1.0                  & 50.3          & 60                & 72.3  \\
                              & \ours                        & \textbf{83.0}                             & \textbf{3.1}                               & \textbf{21.0}                               & \textbf{57.1}                       & \textbf{-2.4}               & \textbf{-6.8}           & \textbf{-0.2}                  & \textbf{-0.9}          & \textbf{58.2}                 & \textbf{-2.9}                         & \textbf{-11.1}                  & \textbf{-0.5}               & \textbf{-1.7}                    & \textbf{68.8}             & \textbf{72.5}                   & \textbf{81.5}  \\

        \bottomrule
    \end{tabular}
    \caption{Single Object Complex Objectives Evaluation}
    \label{tab:comp_result}
\end{table*}

\begin{table*}
    \centering
    \footnotesize
    \setlength\tabcolsep{3pt}
    \begin{tabular}{cc|ccc|ccc|ccc|ccc|ccc|ccc}
        \toprule
        % \multicolumn{2}{c}{} & \multicolumn{18}{c}{Primitive} & \multicolumn{12}{c}{Complex}\\
        \multicolumn{2}{c|}{} & \multicolumn{3}{c|}{up} & \multicolumn{3}{c|}{down} & \multicolumn{3}{c|}{left} & \multicolumn{3}{c|}{right} & \multicolumn{3}{c|}{clock} & \multicolumn{3}{c}{counter}                                                                                                                                                                                                                                                                  \\
        \multicolumn{2}{c|}{} & $S_x^-\uparrow$         & $\Delta x\downarrow$      & $x\downarrow$             & $S_x^+\uparrow$            & $\Delta x\uparrow$         & $x\uparrow$                 & $S_y^-\uparrow$ & $\Delta y\downarrow$ & $y\downarrow$ & $S_y^+\uparrow$ & $\Delta y\uparrow$ & $y\uparrow$ & $S_\theta^-\uparrow$ & $\Delta \theta\downarrow$ & $\theta\downarrow$ & $S_\theta^+\uparrow$ & $\Delta \theta\uparrow$ & $\theta\uparrow$        \\
        \midrule

        \multirow{3}{*}{2D}
                              & Unguided                    & 55.8                       & -0.2                      & -1.3                       & 79.8                        & 0.3                         & 1.3             & 77.1                  & -0.5          & -1.1            & 80.3                &0.5         & 1.3                  & 44.7                       & -1.5               & -3.5                 & 56.4                     & 2.1              & 6.2  \\
                              & Opt.                     & 78.6                       & -0.4                      & -1.0                       & 50.3                        & 0.3                         & 1.0             & 79.2                  & -0.6          & -1.0            & 93.8                & 0.7         & 1.7                  & 46.1                       & \textbf{-2.9}               & -7.8                 & 71.4                     & \textbf{3.5}              & 7.4 \\
                            & \ours                    & \textbf{83.8}             & \textbf{-0.4}            & \textbf{-3.0}             & \textbf{88.1}              & \textbf{0.4}               & \textbf{3.4}   & \textbf{99.3}        & \textbf{-0.7} & \textbf{-2.5}  & \textbf{94.3}      & \textbf{0.7} & \textbf{2.1}        & \textbf{61.3}             & -2.4     & \textbf{-10.5}     & \textbf{68.4}           & 3.3    & \textbf{16.5} \\

        \midrule

        \multirow{3}{*}{3D}
                              & Unguided                    & 40.1                       & -0.1                      & -0.5                       & 40.8                        & 0.1                         & 0.9             & 75.8                  & -0.2          & -0.8            & 87.9                & 0.2         & 0.6                  & 34.7                       & -0.5               & -0.8                 & 29.2                     & 0.1              & 2.5  \\
                              & Opt.                     & 42.4                       & -0.1                      & -0.4                       & 66.4                        & 0.2                         & 1.0            & 77.9                  & -0.2          & -0.4            & 86.6                & 0.3         & 0.8                  & 40.3                       & -1.1               & -1.9                 & 39.2                     & \textbf{1.9}              & 3.5  \\
                            & \ours                    & \textbf{89.7}             & \textbf{-0.2}            & \textbf{-1.5}             & \textbf{66.8}              & \textbf{0.2}               & \textbf{1.2}   & \textbf{96.1}        & \textbf{-0.5} & \textbf{-1.8}  & \textbf{95.4}      & \textbf{0.4} & \textbf{1.3}        & \textbf{69.3}             & \textbf{-2.0}     & \textbf{-5.2}      & \textbf{58.2}           & 1.6    & \textbf{3.5} \\

        \bottomrule
    \end{tabular}
    \caption{Multi-object Primitive Objectives Evaluation}
    \label{tab:multi_prim_result}
\end{table*}

\begin{table*}
    \centering
    \footnotesize
    \setlength\tabcolsep{2pt}
    \begin{tabular}{cc|ccc|ccccc|ccccc}
        \toprule
        % \multicolumn{2}{c}{} & \multicolumn{18}{c}{Primitive} & \multicolumn{12}{c}{Complex}\\
        \multicolumn{2}{c|}{} & \multicolumn{3}{c|}{rotate} & \multicolumn{5}{c|}{clock-up} & \multicolumn{5}{c}{clock-left}                                                                                                                                                                                                                                                                       \\
        \multicolumn{2}{c|}{} & $S_\theta^{+-}\uparrow$      & $|\Delta \theta|\uparrow$     & $|\theta|\uparrow$              & $S_\theta^-\&S_x^-\uparrow$            & $\Delta \theta\downarrow$ & $\theta\downarrow$ & $\Delta x\downarrow$ & $x\downarrow$ & $S_\theta^-\&S_y^+\uparrow$ & $\Delta \theta\downarrow$ & $\theta\downarrow$ & $\Delta y\downarrow$ & $y\downarrow$  \\
        \midrule
        \multirow{3}{*}{2D}
                              & Unguided                        & 68.3                            & 3.2                             & 13.4                            & 35.2                       & -1.5               & -3.5            & -0.2                  & -0.8          & 35.2                 & -1.0                       & -3.0               & -0.5            & -1.0                  \\
                              & Opt.                         & 74.3                            & 3.8                             & 7.2                            & 25.0                       & -1.4               & -0.1            & -0.1                  & -0.2          & 49.0                 & -2.9                       & -4.6               & -0.4             & -0.7                  \\
                            & \ours                        & \textbf{78.4}               & \textbf{4.2}                & \textbf{15.8}               & \textbf{62.4}             & \textbf{-3.3}          & \textbf{-10.6}      & \textbf{-0.4}       & \textbf{-3.6}     & \textbf{63.8}        & \textbf{-3.0}              & \textbf{-6.3}          & \textbf{-0.7}      & \textbf{-2.4}         \\
                            
        \midrule

        \multirow{3}{*}{3D}
                              & Unguided                        & 61.7                             & 2.1                               & 15.8                               & 29.2                       & -0.8               & -0.4            & -0.1                  & -0.5          & 25.2                 & 0.1                         & 2.5                  & -0.2               & -0.7                    \\
                              & Opt.                         & 67.0                            & 2.3                             & 9.5                            & 22.6                       & 0.1                & -0.1            & -0.1                  & -0.3          & 34.3                 & -0.9                       & -1.2               & -0.2            & -0.5                  \\
                                & \ours                        & \textbf{77.6}               & \textbf{2.5}                  & \textbf{21.6}                 & \textbf{44.2}             & \textbf{-1.6}         & \textbf{-7.6}      & \textbf{-0.2}       & \textbf{-1.2}     & \textbf{37.9}        & \textbf{-2.3}               & \textbf{-8.9}          & \textbf{-0.5}      & \textbf{-2.3}          \\

        \bottomrule
    \end{tabular}
    \caption{Multi-object Complex Objectives Evaluation}
    \label{tab:multi_comp_result}
\end{table*}
